# Supplementary material for: Relativistic and electron-correlation effects in static dipole polarizabilities for group 11 elements
Source: arXiv:2410.01493 source file (2025-02-12)
Supplement: Supplementary file 1 [file si.pdf]

# Supporting Information for “Relativistic and Electron-Correlation Effects in Static Dipole Polarizabilities for Group 11 Elements”

YingXing Cheng\*

*Institute of Applied Analysis and Numerical Simulation, University of Stuttgart,  
Pfaffenwaldring 57, 70569, Stuttgart, Germany*

E-mail: [yingxing.cheng@mathematik.uni-stuttgart.de](mailto:yingxing.cheng@mathematik.uni-stuttgart.de)

# Contents

|                                                              |     |
|--------------------------------------------------------------|-----|
| S1 Dipole hyperpolarizabilities obtained by fitting Eq. (S1) | S4  |
| S2 Dipole polarizabilities obtained by fitting Eq. (S2)      | S6  |
| References                                                   | S10 |

Static dipole polarizabilities ( $\alpha$ ) and hyperpolarizabilities ( $\gamma$ ) are computed using the finite-field method 1. The energy of an atom in an external electric field of strength  $F_z$  along the  $z$  axis is given by:

$$E(F_z) \approx E_0 - \frac{1}{2}\alpha F_z^2 - \frac{1}{4!}\gamma F_z^4, \quad (\text{S1})$$

where  $E_0$  is the field-free energy. Least-squares fitting was used to extract  $\alpha$  and  $\gamma$  from computed energies at different field strengths. In cases where  $\gamma$  resulted in unphysical values, only  $\alpha$  was retained using:

$$E(F_z) \approx E_0 - \frac{1}{2}\alpha F_z^2. \quad (\text{S2})$$

A calculation is uniquely identified by a combination of computational method, basis set, and correlation level, represented by a string such as “2C-SR-CC@s-aug-ANO-RCC@(core 3)[vir 279]”. The components of this identifier are separated by the delimiter “@”. The first element refers to the computational method, which can be NR-CC, SR-CC, or DC-CC. The prefix “2C” or “4C” indicates whether the two-component or four-component relativistic Hamiltonian was used, respectively. The second element denotes the basis set used in the calculation. The final element represents the correlation level, which determines the accuracy of the correlated calculations. In this study, the correlation level is described by the number of active electrons and virtual orbitals, expressed as “(core N)[vir M]”, where “N” represents the sum of outer-core and valence electrons, and “M” denotes the number of virtual orbitals. In the coupled-cluster module 2, various correlated methods such as DHF, MP2, CCSD, and CCSD(T) can be employed, all of which follow the same identifier format. The percentage error  $\delta_m$  of a property  $X = \alpha$  or  $\gamma$  is defined as

$$\delta_m = \frac{X_m - X_{\text{CCSD(T)}}}{X_{\text{CCSD(T)}}} \times 100\%, \quad (\text{S3})$$

where  $m$  represents the method used, such as DHF, MP2, or CCSD. For  $X = \gamma$ , the  $\gamma_{\text{CCSD}}$  value is used as the reference in Eq. (S3), instead of  $\gamma_{\text{CCSD(T)}}$ .

## S1 Dipole hyperpolarizabilities obtained by fitting Eq. (S1)

Table S1 lists the  $\gamma$  values for Cu, Ag, and Au obtained by fitting Eq. (S1). All negative  $\gamma$  values are not shown in the table for clarity.

**Table S1: Dipole hyperpolarizability results ( $\gamma$  in  $10^4$  a.u.) for group 11 elements. The error bar represents the uncertainty due to the numerical fitting procedure ( $\Delta P_{\text{fitting}}$ ) for errors greater than 500 a.u.**

| Z  | Atom | State          | $\gamma$ ( $10^4$ a.u.) | $\delta$ (%) | Method  | Comments                                     |
|----|------|----------------|-------------------------|--------------|---------|----------------------------------------------|
| 29 | Cu   | $^2S, M_L = 0$ | 15.81                   | 75.24        | DHF     | 2C-NR-CC@s-aug-dyall.cv4z@(core 29)[vir 299] |
|    |      |                | 36.69                   | 306.71       | MP2     |                                              |
|    |      |                | 6.79                    | -24.70       | CCSD    |                                              |
|    |      |                | 9.02                    | --           | CCSD(T) |                                              |
|    |      | $^2S, M_L = 0$ | 0.97                    | -48.51       | DHF     | 2C-SR-CC@dyall.cv4z@(core 29)[vir 227]       |
|    |      |                | 11.32                   | 499.10       | MP2     |                                              |
|    |      |                | 1.45                    | -23.34       | CCSD    |                                              |
|    |      |                | 1.89                    | --           | CCSD(T) |                                              |
|    |      | $^2S, M_L = 0$ | 14.26                   | 168.55       | DHF     | 2C-SR-CC@s-aug-dyall.cv4z@(core 19)[vir 271] |
|    |      |                | 5.48                    | 3.22         | MP2     |                                              |
|    |      |                | 5.69                    | 7.20         | CCSD    |                                              |
|    |      |                | 5.31                    | --           | CCSD(T) |                                              |
|    |      | $^2S, M_L = 0$ | 14.26                   | 169.69       | DHF     | 2C-SR-CC@s-aug-dyall.cv4z@(core 29)[vir 299] |
|    |      |                | 5.52                    | 4.35         | MP2     |                                              |
|    |      |                | 5.72                    | 8.08         | CCSD    |                                              |
|    |      |                | 5.29                    | --           | CCSD(T) |                                              |
|    |      | $^2S, M_L = 0$ | 17.09                   | 98.10        | DHF     | 2C-SR-CC@d-aug-dyall.cv4z@(core 29)[vir 371] |
|    |      |                | 18.90                   | 118.98       | MP2     |                                              |
|    |      |                | 6.62                    | -23.33       | CCSD    |                                              |
|    |      |                | 8.63                    | --           | CCSD(T) |                                              |
|    |      | $^2S_{1/2}$    | 1.00                    | -28.74       | DHF     | 4C-DC-CC@dyall.cv4z@(core 19)[vir 227]       |
|    |      |                | --                      | --           | MP2     |                                              |
|    |      |                | 1.41                    | --           | CCSD    |                                              |
|    |      | $^2S_{1/2}$    | 14.23                   | 160.75       | DHF     | 4C-DC-CC@s-aug-dyall.cv4z@(core 19)[vir 271] |
|    |      |                | --                      | --           | MP2     |                                              |

(continued)

Table S1. continued.

| Z  | Atom | State          | $\gamma$ ( $10^4$ a.u.) | $\delta$ | Method  | Comments                                     |
|----|------|----------------|-------------------------|----------|---------|----------------------------------------------|
| 47 | Ag   | $^2S, M_L = 0$ | 5.46                    | --       | CCSD    |                                              |
|    |      |                | 28.05                   | 113.10   | DHF     | 2C-NR-CC@s-aug-dyall.cv4z@(core 29)[vir 355] |
|    |      |                | $50.97 \pm 0.01$        | 287.27   | MP2     |                                              |
|    |      |                | 12.85                   | -2.35    | CCSD    |                                              |
|    |      |                | 13.16                   | --       | CCSD(T) |                                              |
|    |      | $^2S, M_L = 0$ | 4.02                    | -9.66    | DHF     | 2C-SR-CC@dyall.cv4z@(core 29)[vir 283]       |
|    |      |                | 20.81                   | 367.91   | MP2     |                                              |
|    |      |                | 3.68                    | -17.25   | CCSD    |                                              |
|    |      |                | 4.45                    | --       | CCSD(T) |                                              |
|    |      | $^2S, M_L = 0$ | 20.01                   | 159.52   | DHF     | 2C-SR-CC@s-aug-dyall.cv4z@(core 29)[vir 355] |
|    |      |                | 23.83                   | 209.05   | MP2     |                                              |
|    |      |                | 8.00                    | 3.77     | CCSD    |                                              |
|    |      |                | 7.71                    | --       | CCSD(T) |                                              |
|    |      | $^2S, M_L = 0$ | 20.00                   | 156.46   | DHF     | 2C-SR-CC@s-aug-dyall.cv4z@(core 19)[vir 331] |
|    |      |                | 24.19                   | 210.13   | MP2     |                                              |
|    |      |                | 8.06                    | 3.35     | CCSD    |                                              |
|    |      |                | 7.80                    | --       | CCSD(T) |                                              |
|    |      | $^2S, M_L = 0$ | 20.13                   | 67.32    | DHF     | 2C-SR-CC@d-aug-dyall.cv4z@(core 29)[vir 427] |
|    |      |                | $122.23 \pm 0.01$       | 916.15   | MP2     |                                              |
|    |      |                | 7.99                    | -33.56   | CCSD    |                                              |
|    |      |                | 12.03                   | --       | CCSD(T) |                                              |
|    |      | $^2S_{1/2}$    | 4.01                    | 6.58     | DHF     | 4C-DC-CC@dyall.cv4z@(core 19)[vir 283]       |
|    |      |                | --                      | --       | MP2     |                                              |
|    |      |                | 3.76                    | --       | CCSD    |                                              |
|    |      | $^2S_{1/2}$    | 19.84                   | 152.71   | DHF     | 4C-DC-CC@s-aug-dyall.cv4z@(core 29)[vir 355] |
|    |      |                | --                      | --       | MP2     |                                              |
|    |      |                | 7.85                    | --       | CCSD    |                                              |
| 79 | Au   | $^2S, M_L = 0$ | 18.24                   | 78.37    | DHF     | 2C-NR-CC@s-aug-dyall.cv4z@(core 43)[vir 381] |
|    |      |                | 43.41                   | 324.47   | MP2     |                                              |
|    |      |                | 9.09                    | -11.11   | CCSD    |                                              |
|    |      |                | 10.23                   | --       | CCSD(T) |                                              |
|    |      | $^2S, M_L = 0$ | 2.49                    | 208.58   | DHF     | 2C-SR-CC@dyall.cv4z@(core 43)[vir 309]       |
|    |      |                | --                      | --       | MP2     |                                              |
|    |      |                | 0.97                    | 19.71    | CCSD    |                                              |
|    |      |                | 0.81                    | --       | CCSD(T) |                                              |
|    |      | $^2S, M_L = 0$ | 5.48                    | 334.09   | DHF     | 2C-SR-CC@s-aug-dyall.cv4z@(core 43)[vir 381] |
|    |      |                | --                      | --       | MP2     |                                              |
|    |      |                | 2.23                    | 76.76    | CCSD    |                                              |

(continued)

Table S1. continued.

| Z | Atom | State          | $\gamma$ ( $10^4$ a.u.) | $\delta$ | Method  | Comments                                     |
|---|------|----------------|-------------------------|----------|---------|----------------------------------------------|
|   |      |                | 1.26                    | --       | CCSD(T) |                                              |
|   |      | $^2S, M_L = 0$ | 5.48                    | 301.56   | DHF     | 2C-SR-CC@s-aug-dyall.cv4z@(core 33)[vir 381] |
|   |      |                | --                      | --       | MP2     |                                              |
|   |      |                | 2.36                    | 72.75    | CCSD    |                                              |
|   |      |                | 1.36                    | --       | CCSD(T) |                                              |
|   |      | $^2S, M_L = 0$ | 5.76                    | -5.36    | DHF     | 2C-SR-CC@d-aug-dyall.cv4z@(core 43)[vir 479] |
|   |      |                | $75.76 \pm 0.01$        | 1145.40  | MP2     |                                              |
|   |      |                | 2.87                    | -52.84   | CCSD    |                                              |
|   |      |                | 6.08                    | --       | CCSD(T) |                                              |
|   |      | $^2S_{1/2}$    | 2.39                    | 106.58   | DHF     | 4C-DC-CC@dyall.cv4z@(core 33)[vir 309]       |
|   |      |                | --                      | --       | MP2     |                                              |
|   |      |                | 1.16                    | --       | CCSD    |                                              |
|   |      | $^2S_{1/2}$    | 5.22                    | 118.12   | DHF     | 4C-DC-CC@s-aug-dyall.cv4z@(core 33)[vir 381] |
|   |      |                | --                      | --       | MP2     |                                              |
|   |      |                | 2.39                    | --       | CCSD    |                                              |

Table S2 summarizes the highlighted  $\gamma$  results for group 11 elements in Table S1.

**Table S2: Static hyperpolarizabilities (in  $10^4$  a.u.) with nonrelativistic, scalar-relativistic, full Dirac-Coulomb relativistic effects of group 11 elements.**

| $\hat{H}$ | State       | Method  | Cu              | Ag               | Au               |
|-----------|-------------|---------|-----------------|------------------|------------------|
| NR        | $^2S$       | DHF     | 15.81           | $28.05 \pm 0.20$ | $18.24 \pm 0.52$ |
|           |             | CCSD    | 6.79            | $12.85 \pm 0.20$ | $9.09 \pm 0.52$  |
|           |             | CCSD(T) | $9.02 \pm 0.37$ | $13.16 \pm 0.24$ | $10.23 \pm 0.61$ |
| $SR_n$    | $^2S$       | DHF     | 14.26           | 20.01            | 5.48             |
|           |             | CCSD    | 5.72            | 8.00             | 2.23             |
|           |             | CCSD(T) | $5.29 \pm 0.19$ | $7.71 \pm 0.06$  | $1.26 \pm 0.36$  |
| $SR_d$    | $^2S$       | DHF     | 14.26           | 20.01            | 5.48             |
|           |             | CCSD    | 5.69            | 8.00             | 2.36             |
|           |             | CCSD(T) | $5.31 \pm 0.06$ | $7.71 \pm 0.06$  | $1.36 \pm 0.19$  |
| DC        | $^2S_{1/2}$ | DHF     | 14.23           | 19.84            | 5.22             |
|           |             | CCSD    | 5.46            | 7.85             | 2.39             |
|           |             | CCSD(T) | --              | --               | --               |

## S2 Dipole polarizabilities obtained by fitting Eq. (S2)

Table S3 lists all results for Cu, Ag, and Au obtained by fitting Eq. (S2).

**Table S3: Dipole polarizability results ( $\alpha$  in a.u.) for group 11 elements. The error bar represents the uncertainty due to the numerical fitting procedure ( $\Delta P_{\text{fitting}}$ ) for errors greater than 0.005 a.u.**

| Z  | Atom | State          | $\alpha$ (a.u.)   | $\delta$ (%) | Method  | Comments                                     |
|----|------|----------------|-------------------|--------------|---------|----------------------------------------------|
| 29 | Cu   | $^2S, M_L = 0$ | $77.50 \pm 0.03$  | 53.83        | DHF     | 2C-NR-CC@s-aug-dyall.cv4z@(core 29)[vir 299] |
|    |      |                | $32.36 \pm 0.06$  | -35.78       | MP2     |                                              |
|    |      |                | $53.65 \pm 0.01$  | 6.47         | CCSD    |                                              |
|    |      |                | $50.38 \pm 0.01$  | --           | CCSD(T) |                                              |
|    |      | $^2S, M_L = 0$ | 70.60             | 53.76        | DHF     | 2C-SR-CC@dyall.cv4z@(core 29)[vir 227]       |
|    |      |                | $29.15 \pm 0.02$  | -36.52       | MP2     |                                              |
|    |      |                | 48.98             | 6.67         | CCSD    |                                              |
|    |      |                | 45.91             | --           | CCSD(T) |                                              |
|    |      | $^2S, M_L = 0$ | $71.06 \pm 0.02$  | 52.41        | DHF     | 2C-SR-CC@s-aug-dyall.cv4z@(core 19)[vir 271] |
|    |      |                | $29.04 \pm 0.01$  | -37.71       | MP2     |                                              |
|    |      |                | $49.52 \pm 0.01$  | 6.21         | CCSD    |                                              |
|    |      |                | $46.62 \pm 0.01$  | --           | CCSD(T) |                                              |
|    |      | $^2S, M_L = 0$ | $71.06 \pm 0.02$  | 52.25        | DHF     | 2C-SR-CC@s-aug-dyall.cv4z@(core 29)[vir 299] |
|    |      |                | $29.12 \pm 0.01$  | -37.60       | MP2     |                                              |
|    |      |                | $49.64 \pm 0.01$  | 6.36         | CCSD    |                                              |
|    |      |                | $46.67 \pm 0.01$  | --           | CCSD(T) |                                              |
|    |      | $^2S, M_L = 0$ | $71.12 \pm 0.03$  | 52.40        | DHF     | 2C-SR-CC@d-aug-dyall.cv4z@(core 29)[vir 371] |
|    |      |                | $28.94 \pm 0.03$  | -37.99       | MP2     |                                              |
|    |      |                | $49.66 \pm 0.01$  | 6.41         | CCSD    |                                              |
|    |      |                | $46.67 \pm 0.01$  | --           | CCSD(T) |                                              |
|    |      | $^2S_{1/2}$    | 70.51             | 52.79        | DHF     | 4C-DC-CC@dyall.cv4z@(core 19)[vir 227]       |
|    |      |                | $31.64 \pm 0.47$  | -31.43       | MP2     |                                              |
|    |      |                | 48.91             | 6.00         | CCSD    |                                              |
|    |      |                | $46.15 \pm 0.06$  | --           | CCSD(T) |                                              |
|    |      | $^2S_{1/2}$    | $70.97 \pm 0.02$  | 50.96        | DHF     | 4C-DC-CC@s-aug-dyall.cv4z@(core 19)[vir 271] |
|    |      |                | $33.12 \pm 1.67$  | -29.55       | MP2     |                                              |
|    |      |                | $49.47 \pm 0.01$  | 5.23         | CCSD    |                                              |
|    |      |                | $47.01 \pm 0.17$  | --           | CCSD(T) |                                              |
| 47 | Ag   | $^2S, M_L = 0$ | $106.09 \pm 0.05$ | 68.58        | DHF     | 2C-NR-CC@s-aug-dyall.cv4z@(core 29)[vir 355] |
|    |      |                | $32.64 \pm 0.08$  | -48.14       | MP2     |                                              |
|    |      |                | $68.37 \pm 0.02$  | 8.63         | CCSD    |                                              |
|    |      |                | $62.93 \pm 0.02$  | --           | CCSD(T) |                                              |
|    |      | $^2S, M_L = 0$ | $81.90 \pm 0.01$  | 61.37        | DHF     | 2C-SR-CC@dyall.cv4z@(core 29)[vir 283]       |
|    |      |                | $27.01 \pm 0.03$  | -46.78       | MP2     |                                              |
|    |      |                | $54.65 \pm 0.01$  | 7.68         | CCSD    |                                              |
|    |      |                | $50.76 \pm 0.01$  | --           | CCSD(T) |                                              |

(continued)

Table S3. continued.

| Z  | Atom | State          | $\alpha$ (a.u.)   | $\delta$ | Method  | Comments                                     |
|----|------|----------------|-------------------|----------|---------|----------------------------------------------|
|    |      | $^2S, M_L = 0$ | $82.32 \pm 0.03$  | 61.56    | DHF     | 2C-SR-CC@s-aug-dyall.cv4z@(core 29)[vir 355] |
|    |      |                | $26.26 \pm 0.04$  | -48.45   | MP2     |                                              |
|    |      |                | $54.89 \pm 0.01$  | 7.73     | CCSD    |                                              |
|    |      |                | $50.95 \pm 0.01$  | --       | CCSD(T) |                                              |
|    |      | $^2S, M_L = 0$ | $82.32 \pm 0.03$  | 60.40    | DHF     | 2C-SR-CC@s-aug-dyall.cv4z@(core 19)[vir 331] |
|    |      |                | $27.46 \pm 0.04$  | -46.50   | MP2     |                                              |
|    |      |                | $55.16 \pm 0.01$  | 7.47     | CCSD    |                                              |
|    |      |                | $51.32 \pm 0.01$  | --       | CCSD(T) |                                              |
|    |      | $^2S, M_L = 0$ | $82.32 \pm 0.03$  | 61.62    | DHF     | 2C-SR-CC@d-aug-dyall.cv4z@(core 29)[vir 427] |
|    |      |                | $25.91 \pm 0.2$   | -49.14   | MP2     |                                              |
|    |      |                | $54.89 \pm 0.01$  | 7.77     | CCSD    |                                              |
|    |      |                | $50.93 \pm 0.02$  | --       | CCSD(T) |                                              |
|    |      | $^2S_{1/2}$    | $81.71 \pm 0.01$  | 59.53    | DHF     | 4C-DC-CC@dyall.cv4z@(core 19)[vir 283]       |
|    |      |                | $30.92 \pm 0.5$   | -39.62   | MP2     |                                              |
|    |      |                | $54.91 \pm 0.01$  | 7.20     | CCSD    |                                              |
|    |      |                | $51.22 \pm 0.03$  | --       | CCSD(T) |                                              |
|    |      | $^2S_{1/2}$    | $82.12 \pm 0.03$  | 60.61    | DHF     | 4C-DC-CC@s-aug-dyall.cv4z@(core 29)[vir 355] |
|    |      |                | $31.31 \pm 1.87$  | -38.77   | MP2     |                                              |
|    |      |                | $54.79 \pm 0.01$  | 7.16     | CCSD    |                                              |
|    |      |                | $51.13 \pm 0.09$  | --       | CCSD(T) |                                              |
| 79 | Au   | $^2S, M_L = 0$ | $107.03 \pm 0.03$ | 70.67    | DHF     | 2C-NR-CC@s-aug-dyall.cv4z@(core 43)[vir 381] |
|    |      |                | $27.14 \pm 0.07$  | -56.73   | MP2     |                                              |
|    |      |                | $68.51 \pm 0.01$  | 9.25     | CCSD    |                                              |
|    |      |                | $62.71 \pm 0.02$  | --       | CCSD(T) |                                              |
|    |      | $^2S, M_L = 0$ | 48.11             | 33.28    | DHF     | 2C-SR-CC@dyall.cv4z@(core 43)[vir 309]       |
|    |      |                | 24.52             | -32.08   | MP2     |                                              |
|    |      |                | 37.43             | 3.68     | CCSD    |                                              |
|    |      |                | 36.10             | --       | CCSD(T) |                                              |
|    |      | $^2S, M_L = 0$ | $48.38 \pm 0.01$  | 32.71    | DHF     | 2C-SR-CC@s-aug-dyall.cv4z@(core 43)[vir 381] |
|    |      |                | $24.62 \pm 0.02$  | -32.46   | MP2     |                                              |
|    |      |                | 37.75             | 3.55     | CCSD    |                                              |
|    |      |                | 36.46             | --       | CCSD(T) |                                              |
|    |      | $^2S, M_L = 0$ | $48.38 \pm 0.01$  | 32.22    | DHF     | 2C-SR-CC@s-aug-dyall.cv4z@(core 33)[vir 381] |
|    |      |                | $25.11 \pm 0.02$  | -31.37   | MP2     |                                              |
|    |      |                | 37.91             | 3.60     | CCSD    |                                              |
|    |      |                | 36.59             | --       | CCSD(T) |                                              |
|    |      | $^2S, M_L = 0$ | $48.39 \pm 0.01$  | 33.12    | DHF     | 2C-SR-CC@d-aug-dyall.cv4z@(core 43)[vir 479] |
|    |      |                | $24.20 \pm 0.23$  | -33.43   | MP2     |                                              |

(continued)



Table S3. continued.

| Z | Atom | State       | $\alpha$ (a.u.)  | $\delta$ | Method  | Comments                                     |
|---|------|-------------|------------------|----------|---------|----------------------------------------------|
|   |      |             | 37.68            | 3.65     | CCSD    |                                              |
|   |      |             | $36.35 \pm 0.01$ | --       | CCSD(T) |                                              |
|   |      | $^2S_{1/2}$ | 47.87            | 31.19    | DHF     | 4C-DC-CC@dyall.cv4z@(core 33)[vir 309]       |
|   |      |             | $30.62 \pm 3.72$ | -16.08   | MP2     |                                              |
|   |      |             | 37.55            | 2.91     | CCSD    |                                              |
|   |      |             | $36.49 \pm 0.18$ | --       | CCSD(T) |                                              |
|   |      | $^2S_{1/2}$ | $48.16 \pm 0.01$ | 31.20    | DHF     | 4C-DC-CC@s-aug-dyall.cv4z@(core 33)[vir 381] |
|   |      |             | $27.17 \pm 0.87$ | -25.96   | MP2     |                                              |
|   |      |             | 37.89            | 3.24     | CCSD    |                                              |
|   |      |             | $36.70 \pm 0.05$ | --       | CCSD(T) |                                              |

Table S4 summarizes the most accurate  $\alpha$  results for group 11 elements in Table S3 from Eq. (S2).

**Table S4: Static dipole polarizabilities (in a.u.) with nonrelativistic, scalar-relativistic, and full Dirac-Coulomb relativistic effects for group 11 elements.**  $SR_n$  represents the SR results obtained using the same correlation level as in the NR calculations, while  $SR_d$  represents the SR results evaluated using the same correlation level as in the DC calculations. The error due to the numerical fitting procedure ( $\Delta P_{\text{fitting}}$ ) is shown as the error bar. The recommended values from Ref. 3 are also listed.

| $\hat{H}$ | State       | Method  | Cu               | Ag                | Au                |
|-----------|-------------|---------|------------------|-------------------|-------------------|
| NR        | $^2S$       | DHF     | $77.50 \pm 0.03$ | $106.09 \pm 0.05$ | $107.03 \pm 0.03$ |
|           |             | CCSD    | $53.65 \pm 0.03$ | $68.37 \pm 0.05$  | $68.51 \pm 0.03$  |
|           |             | CCSD(T) | $50.38 \pm 0.01$ | $62.93 \pm 0.02$  | $62.71 \pm 0.02$  |
| $SR_n$    | $^2S$       | DHF     | $71.06 \pm 0.02$ | $82.32 \pm 0.03$  | $48.38 \pm 0.01$  |
|           |             | CCSD    | $49.64 \pm 0.02$ | $54.89 \pm 0.03$  | $37.75 \pm 0.01$  |
|           |             | CCSD(T) | $46.67 \pm 0.01$ | $50.95 \pm 0.01$  | 36.46             |
| $SR_d$    | $^2S$       | DHF     | $71.06 \pm 0.02$ | $82.32 \pm 0.03$  | $48.38 \pm 0.01$  |
|           |             | CCSD    | $49.52 \pm 0.02$ | $54.89 \pm 0.03$  | $37.91 \pm 0.01$  |
|           |             | CCSD(T) | $46.62 \pm 0.01$ | $50.95 \pm 0.01$  | 36.59             |
| DC        | $^2S_{1/2}$ | DHF     | $70.97 \pm 0.02$ | $82.12 \pm 0.03$  | $48.16 \pm 0.01$  |
|           |             | CCSD    | $49.47 \pm 0.02$ | $54.79 \pm 0.03$  | $37.89 \pm 0.01$  |
|           |             | CCSD(T) | $47.01 \pm 0.17$ | $51.13 \pm 0.09$  | $36.70 \pm 0.05$  |
| Ref. 3    | --          | --      | $46.5 \pm 0.5$   | $55.0 \pm 8$      | $36.0 \pm 3$      |

## References

- (1) Das, A. K.; Thakkar, A. J. Static Response Properties of Second-Period Atoms: Coupled Cluster Calculations. *J. Phys. B At. Mol. Opt. Phys.* **1998**, *31*, 2215.
- (2) DIRAC18. <https://doi.org/10.5281/zenodo.2253986>, Accessed on Jun 7, 2021.
- (3) Schwerdtfeger, P.; Nagle, J. K. 2018 Table of Static Dipole Polarizabilities of the Neutral Elements in the Periodic Table. *Mol. Phys.* **2019**, *117*, 1200–1225.
